# Supplementary material for: Action-guided generation of 3D functionality segmentation data
Source: arXiv:2511.23230 source file (2026-04-04)
Supplement: Supplementary file 2 [file mypackages.tex]

\usepackage{algorithmic}
\usepackage{array}
\usepackage{textcomp}
\usepackage{stfloats}
\usepackage{url}
\usepackage{graphicx}
\usepackage{amsmath,amssymb,amsfonts}
\usepackage{multirow,multicol}
\usepackage[T1]{fontenc}
\usepackage[accsupp]{axessibility}
\usepackage{microtype}
\usepackage{balance}
\usepackage{wrapfig,booktabs}
\usepackage{overpic}
\usepackage{pifont}
\usepackage{tikz}
\usepackage{pgfplots}
\usepackage{comment}
\usepackage{soul}
\usepackage[x11names]{xcolor}
\pgfplotsset{compat=1.18}
\usepgfplotslibrary{groupplots}
\usepackage{pgfplots}
\usepackage{pgfmath}
\usepackage{todonotes}
\usepackage{comment}

%\usepackage[justification=raggedright,singlelinecheck=false]{caption}
% \pgfplotsset{every axis/.append style={
%     title={\small \textbf{Overall Preference}},
%     title style={at={(0.5,1)}, anchor=south, yshift=0pt},
%     ymin=0, ymax=100,
%     ybar stacked, bar width=15pt,
%     xtick=data,
%     ytick={},
%     yticklabels={},
%     grid=major,
%     major grid style={line width=0.3pt, gray!30},
%     axis x line=bottom,
%     axis y line=left,
%     axis line style = {draw=none},
%     x tick label style={rotate=0, anchor=north},
%     enlarge x limits=0.35,
%     nodes near coords={\pgfmathprintnumber{\pgfplotspointmeta}\%},
%     every node near coord/.append style={font=\tiny, text=black},
%     width=3cm, height=4cm,
%     tick label style={font=\small},
% }}

\usepackage{xcolor}
\definecolor{lightgraybg}{RGB}{245,245,245}
\definecolor{deepgrayborder}{RGB}{120,120,120}
\usepackage[table]{xcolor}
\definecolor{verylightpink}{HTML}{FFD6D6}
\definecolor{brightgreen}{RGB}{0,176,80}

\usepackage{listings}
\lstset{
    escapeinside={(*}{*)},
    breaklines=true, 
    breakatwhitespace=true, 
    breakautoindent=false,
    backgroundcolor=\color{lightgraybg}, 
    frame=single,
    rulecolor=\color{deepgrayborder}, 
    framerule=1.2pt, 
}

\usepackage{tabularx}
